# Supplementary material for: Competing Time Scales Lead to Oscillations in Shear-Thickening Suspensions
Source: arXiv:1902.07655 ancillary file (2019-07-22)
Supplement: Supplementary file 1 [file Supplemental_Material_v2.pdf]

# Supplemental Material: Competing Time Scales Lead to Oscillations in Shear-Thickening Suspensions

J. A. Richards,<sup>1,\*</sup> J. R. Royer,<sup>1</sup> B. Liebchen,<sup>1,2</sup> B. M. Guy,<sup>1</sup> and W. C. K. Poon<sup>1</sup>

<sup>1</sup>*SUPA, School of Physics and Astronomy, The University of Edinburgh, King's Buildings, Peter Guthrie Tait Road, Edinburgh EH9 3FD, United Kingdom*

<sup>2</sup>*Institut für Theoretische Physik II: Weiche Materie, Heinrich-Heine-Universität Düsseldorf, D-40225 Düsseldorf, Germany*

(Dated: July 22, 2019)

In §S1, we derive the linear stability criterion. In §S2, the experimental data for the 50 wt.% glycerol-water cornstarch suspension is compared to the WC model. In §S3, we derive the equivalent areal density for parallel disk flow. In §S4, the strain scale for thickening,  $\gamma_0$ , is estimated from controlled-rate experiments. In §S5, flow curves for tuned cornstarch and silica systems are shown. In §S6 the effect of reducing gap height is outlined. In §S7, the process for estimation of  $t_r$  is outlined. Finally in §S8, the behavior at the onset of oscillation is detailed.

## S1. LINEAR STABILITY ANALYSIS

The Jacobian,  $J$ , describing the phase-plane behavior, is given by

$$J = \begin{bmatrix} \frac{\partial g_1}{\partial \Gamma} & \frac{\partial g_1}{\partial f} \\ \frac{\partial g_2}{\partial \Gamma} & \frac{\partial g_2}{\partial f} \end{bmatrix} = \begin{bmatrix} -\eta_r & -\dot{\Gamma} \frac{d\eta_r}{df} \\ \frac{\dot{\Gamma}}{\epsilon} \frac{\partial \hat{f}}{\partial \Gamma} & \frac{\dot{\Gamma}}{\epsilon} \left( \frac{\partial \hat{f}}{\partial f} - 1 \right) \end{bmatrix} = \begin{bmatrix} -\eta_r & -\dot{\Gamma} \frac{d\eta_r}{df} \\ \frac{\dot{\Gamma} \eta_r}{\epsilon} \frac{d\hat{f}}{d\Sigma} & \frac{\dot{\Gamma}}{\epsilon} \left( \dot{\Gamma} \frac{d\eta_r}{df} \frac{d\hat{f}}{d\Sigma} - 1 \right) \end{bmatrix}. \quad (\text{S1})$$

Evaluating  $J$  at the fixed point, this simplifies to

$$\begin{bmatrix} -\eta_r & -\dot{\Gamma} \frac{d\eta_r}{df} \\ \frac{\dot{\Gamma} \eta_r}{\epsilon} \frac{d\hat{f}}{d\Sigma_E} & \frac{\dot{\Gamma}}{\epsilon} \left( \dot{\Gamma} \frac{d\eta_r}{d\Sigma_E} - 1 \right) \end{bmatrix}, \quad (\text{S2})$$

with expressions from Eqs. 1-3 in dimensionless form and where derivatives are evaluated at the fixed point ( $g_2 = 0$ ,  $g_1 = 0$ ). The behavior about the fixed point is determined by the eigenvalues of the matrix,  $\lambda_{1,2}$ , given by the roots of the equation

$$\epsilon \lambda^2 + \lambda \frac{\eta_r}{\dot{\Gamma}} \left( \epsilon + \frac{\dot{\Gamma}}{\eta_r} \left( 1 - \dot{\Gamma} \frac{d\eta_r}{d\Sigma_E} \right) \right) + \frac{\eta_r}{\dot{\Gamma}} = 0. \quad (\text{S3})$$

When the real part of either  $\lambda$  is positive,  $\Re(\lambda) > 0$ , the fixed point becomes unstable.

There are now two possibilities for the solution to this equation in the form,  $a\lambda^2 + b\lambda + c = 0$ ,  $\lambda_{1,2} = (-b \pm \sqrt{b^2 - 4ac})/2a$ . Firstly,  $b^2 - 4ac < 0$ : the fixed point becomes unstable when  $b$  becomes negative;  $\Re(\lambda_1), \Re(\lambda_2) > 0$  and a sink becomes a source. Secondly  $b^2 - 4ac > 0$ , *i.e.*, the fixed point becomes unstable when only  $\Re(\lambda_1) > 0$  and the sink becomes a saddle point. In the latter case, this requires:  $-b + \sqrt{b^2 - 4ac} > 0$ , or  $-4ac > 0$ . However, as  $a = \epsilon$  and  $c = \eta_r/\dot{\Gamma}$  are strictly positive, this condition is not possible. We therefore return to the first case: the fixed point becomes unstable when  $b < 0$ . The instability criterion is then

$$\frac{\eta_r}{\dot{\Gamma}} \left( \epsilon + \frac{\dot{\Gamma}}{\eta_r} \left( 1 - \dot{\Gamma} \frac{d\eta_r}{d\Sigma_E} \right) \right) < 0,$$

$$\epsilon < \frac{\dot{\Gamma}}{\eta_r} \left( \dot{\Gamma} \frac{d\eta_r}{d\Sigma_E} - 1 \right) = \dot{\Gamma} \left( \frac{\Sigma_E}{\eta_r^2} \frac{d\eta_r}{d\Sigma_E} - \frac{1}{\eta_r} \right) = -\dot{\Gamma} \frac{d}{d\Sigma_E} \left( \frac{\Sigma_E}{\eta_r} \right).$$

Written finally as

$$\epsilon < -\dot{\Gamma} \frac{d\dot{\Gamma}}{d\Sigma_E}. \quad (\text{S4})$$

This result, as both  $\Re(\lambda)$  become positive simultaneously, also means that all bifurcations must be Hopf bifurcations.

---

\* jamesrichards92@gmail.com

## S2. COMPARISON WITH THE WC MODEL

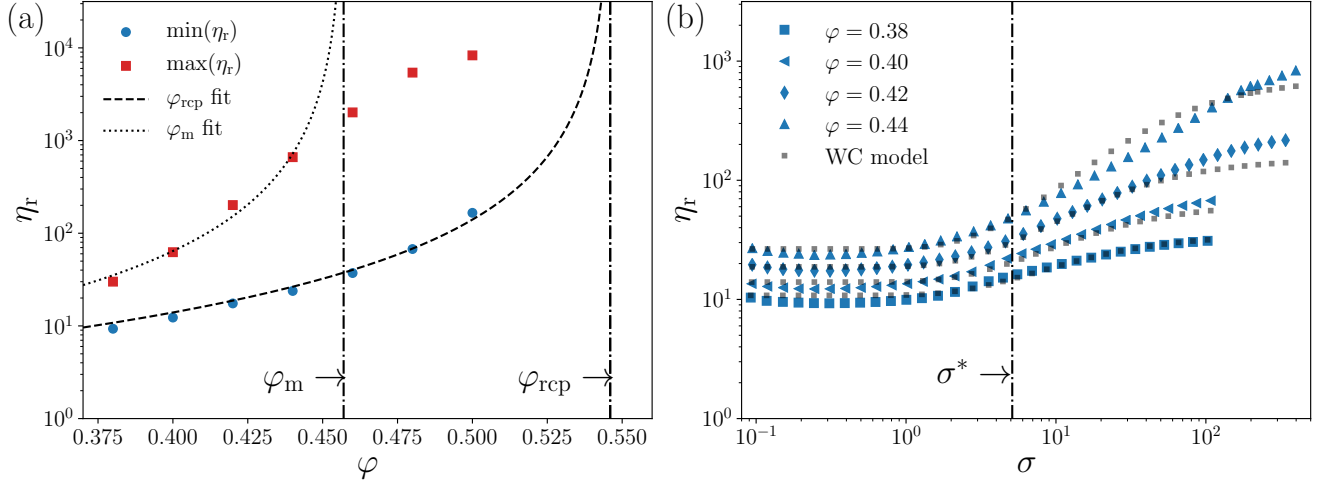

FIG. S1. Fitting of the WC model to 50 wt.% glycerol-water cornstarch suspension rheology. (a) Limiting viscosity states. Solid points: experimental minimum and maximum relative viscosities,  $\eta_r$ , as a function of weight fraction,  $\varphi$ . Dashed and dotted lines are fits to Eq. S5 for  $\min \eta_r$  and  $\max \eta_r$  respectively, finding  $\varphi_{rcp} = 0.546 \pm 0.002$  and  $\varphi_m = 0.457 \pm 0.001$ . (b) Corrected steady state rheological data (blue) and WC model fit (black), with  $\beta = 0.94 \pm 0.03$  and  $\sigma^* = 5.1 \pm 0.3$ .

Using data from the time-averaged flow curves, Fig. 1(a), the limiting jamming weight fractions,  $\varphi_{rcp}$  and  $\varphi_m$ , are found from fitting (least squares in logarithmic space) respectively the minimum viscosity for all  $\varphi$  measured and the maximum viscosity for  $\varphi \leq 0.44$  (for which a steady maximum viscosity is found) to the Quemada equation,

$$\eta_r = \left[ 1 - \frac{\varphi}{\varphi_J} \right]^{-2}, \quad (S5)$$

Fig. S1(a), finding  $\varphi_{rcp} = 0.546 \pm 0.002$  and  $\varphi_m = 0.457 \pm 0.001$ . Fixing these values,  $\beta$  and  $\sigma^*$  are found from fitting steady-state data for  $\varphi \leq 0.44$ , to which a non-Newtonian correction for parallel-plate measurements has been applied,

$$\sigma = \frac{\mathcal{T}_E}{2\pi R^3} \left( 3 + \frac{d \ln \mathcal{T}_E}{d \ln \Omega} \right), \quad (S6)$$

Fig. S1(b). We find  $\beta = 0.94 \pm 0.03$  and  $\sigma^* = 5.1 \pm 0.3$ . As the shear-rate derivative can become negative and the shear rate time dependent at higher  $\varphi$ , we report apparent stresses for all other results unless explicitly stated. All data for cornstarch suspensions is reported for increasing stress, however reversibility of shear-thickening below sample fracture was checked, Fig. S2.

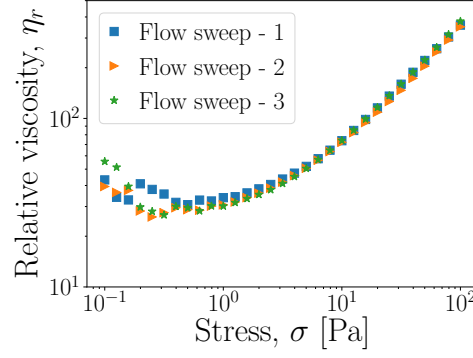

FIG. S2. Reversibility of shear thickening at  $\varphi = 0.43$ . Repeated controlled-stress flow sweeps between 0.1 Pa and 100 Pa for a cornstarch suspension in 50 wt.% glycerol. Flow sweep - 1, increasing stress; Flow sweep - 2, decreasing stress; and Flow sweep - 3, increasing stress. See legend for symbols.

### S3. CONVERTING GEOMETRY INERTIA FROM PARALLEL DISK TO RECTILINEAR FLOW

We begin with the rotational equation of motion for the geometry with moment of inertia,  $I$ , and angular velocity  $\Omega$ :

$$I \frac{d\Omega}{dt} = \mathcal{T}_E - \mathcal{T}_{\text{sample}}, \quad (\text{S7})$$

with the applied torque from the rheometer ( $\mathcal{T}_E$ ) and the sample torque ( $\mathcal{T}$ ) resisting this. With a radius  $R$  and gap height  $h$ , using the definition for the rim shear rate ( $\dot{\gamma} = \Omega R/h$ ) and apparent stress ( $\sigma = \eta \dot{\gamma} = 2\mathcal{T}/\pi R^3$ ) the equivalent areal density,  $\rho_A$ , is unambiguously defined:

$$\begin{aligned} I \frac{d}{dt} \left( \frac{\dot{\gamma} h}{R} \right) &= \frac{\pi R^3}{2} (\sigma_E - \eta \dot{\gamma}) \\ \underbrace{\left( \frac{2I}{\pi R^4} \right)}_{\rho_A} h \frac{d\dot{\gamma}}{dt} &= \sigma_E - \eta \dot{\gamma}. \end{aligned} \quad (\text{S8})$$

The choice of rim shear rate and apparent stress was made following Ref. [1].

#### S4. FRICTIONAL CONTACT DYNAMICS UNDER IMPOSED STRAIN

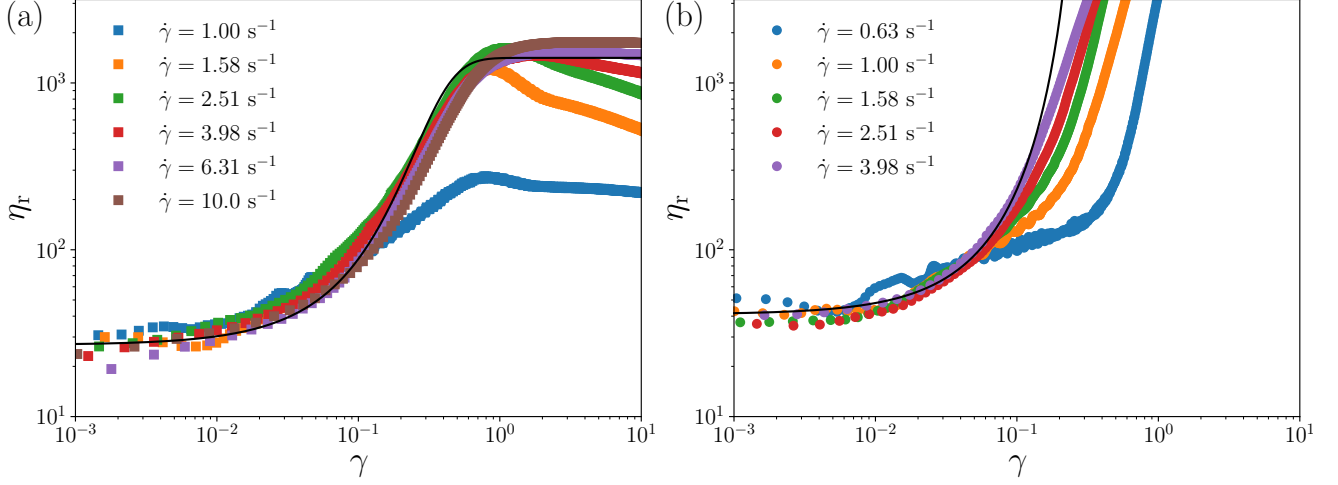

FIG. S3. Strain-dependent viscosity response under imposed shear rate,  $\dot{\gamma}$ : relative viscosity,  $\eta_r$  vs. rim strain,  $\gamma$ . (a)  $\phi = 0.44$  cornstarch suspension in 85 wt.% glycerol-water, response on changing  $\dot{\gamma}$  from  $0.01 \text{ s}^{-1}$ , solid squares, see legend for  $\dot{\gamma}$ . Black line: model using Eq. S9, parameters from §S5B and Eqs. 1-3 with  $\gamma_0 = 0.12$ , estimated by eye. Note, the viscosity trace is shifted vertically by a factor of 0.4 to aid the eye, as we are interested in the *strain* at which  $\eta_r$  changes, *i.e.* minimizing the error in  $\gamma$  only. (b)  $\phi = 0.46$ , otherwise as (a).

To separately measure the strain scale for the response of the frictional contact network,  $\gamma_0$ , see Eq. 4, the strain-dependent response of the viscosity,  $\eta_r(\gamma)$ , to changes in stress needs to be made without introducing additional dynamics. One possible way is under imposed stress, with a geometry inertial time-scale shorter than the contact network formation time, *i.e.*  $\epsilon \gtrsim 1$ . As  $h$ ,  $\sigma^*$  and  $\rho_A$  are relatively fixed, only  $\eta_s$  can be freely varied, but this criterion would require a very high background solvent viscosity *e.g.*  $\eta_s \gtrsim 1 \text{ Pa s}$ . It is also possible to measure  $\eta_r(\gamma)$  under imposed rate, here  $t_c$  needs to be reduced below the response time for changes in the shear rate. With a response time of  $\sim 0.02 \text{ s}$  for the ARES-G2, this requires  $\eta_s$  to be of the order of 100 mPa s.

We therefore use a cornstarch suspension in an 85 wt.% glycerol-water background solvent to measure an estimate of  $\gamma_0$ , with  $\eta_s = 75 \text{ mPa s}$  measured from centrifuged sample supernatant. Measurements on the suspension were made under imposed rate, using a TA Instruments ARES-G2 rheometer, with cross-hatched parallel plates ( $R = 20 \text{ mm}$  and  $h = 1 \text{ mm}$ ), reporting rim shear rates and apparent viscosity as a function of rim strain,  $\gamma$ . Due to the high noise level for rapid transient measurements a large change in viscosity is required;  $\phi \gtrsim \phi_{\text{DST}}$  are therefore used.

To develop the microstructure in the direction of shear in the frictionless state the suspension is sheared at  $0.01 \text{ s}^{-1}$ , far below the onset of shear thickening. The shear rate is then ‘jumped’ to a higher rate, above the DST shear rate, typically  $> 1 \text{ s}^{-1}$ , and the response is measured for  $\gamma \sim 10$ , Fig. S4. The evolution of the viscosity will depend in general on both strain and sample stress, but in jumping to a large shear rate, where the sample stress is immediately much greater than  $\sigma^*$ , Eq. 4 reduces to

$$f(\gamma) = 1 - \exp\left(-\frac{\gamma}{\gamma_0}\right). \quad (\text{S9})$$

The viscosity is then also only a function of strain, using Eqs. 2 & 3. In Fig. S4, we show data for  $\phi = 0.44$ , Fig. S4(a), and  $\phi = 0.46$ , Fig. S4(b), compared to  $\eta_r$  from Eq. S9, finding  $\gamma_0 \approx 0.12$ . No strong  $\phi$  dependence is apparent around  $\phi_m$ , although we note that the data for  $\phi = 0.46$  is complicated by sample edge fracture soon after thickening begins.

## S5. ADDITIONAL STEADY-STATE RHEOLOGICAL DATA

### A. Cornstarch in 67 wt. % glycerol

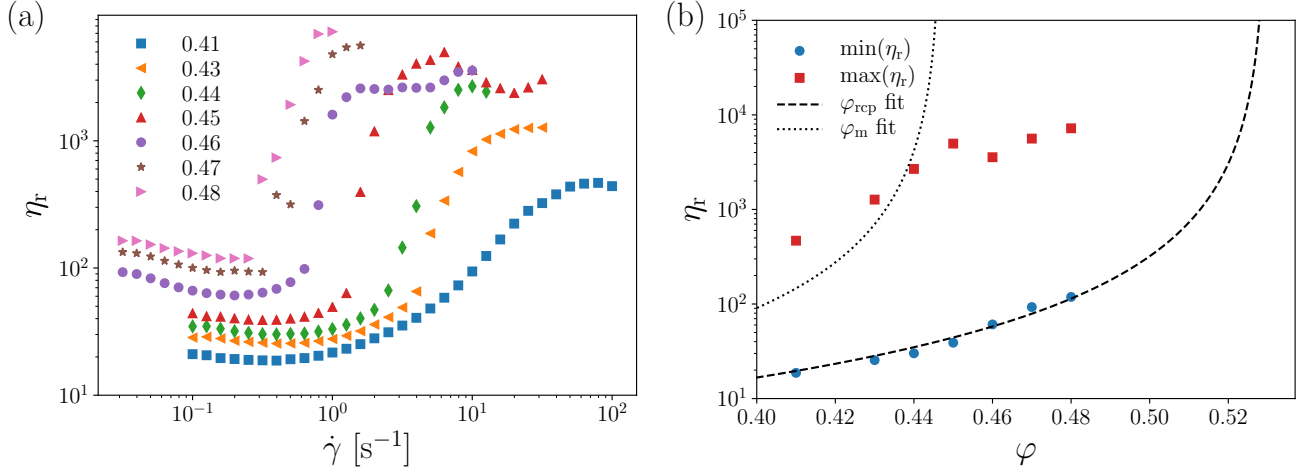

FIG. S4. Steady-state shear rheology of a cornstarch suspension in 67 wt.% glycerol-water background solvent. (a) Relative viscosity,  $\eta_r$ , *vs.* shear rate,  $\dot{\gamma}$  for multiple weight fractions,  $\phi$  listed. (b) Maximum (red squares) and minimum (blue circles) viscosities as a function of  $\phi$ , fits to Eq. S5 are shown, dotted and dashed black lines respectively, finding  $\phi_m = 0.447 \pm 0.003$  and  $\phi_{rcp} = 0.530 \pm 0.002$ .

Cornstarch (Sigma Aldrich, particle diameter  $\approx 14 \mu\text{m}$  and polydispersity  $\approx 40\%$  from static light scattering [1]) was dispersed into 67 wt.% glycerol-water ( $\eta_s = 17 \text{ mPa}\cdot\text{s}$ , measured from centrifuged suspension supernatant). Samples were rested for  $\sim 1 \text{ h}$  on a roller bank before measurement. Steady-state flow curves were measured using a TA Instruments ARES-G2 with sandblasted parallel plates ( $R = 20 \text{ mm}$  and  $h = 1 \text{ mm}$ ). We report rim shear rates and apparent viscosities. Measurements were taken under imposed shear rate from  $0.1 \text{ s}^{-1}$  for  $\phi \leq 0.45$  or  $0.0316 \text{ s}^{-1}$  for  $\phi \geq 0.46$  till fracture with a single up-sweep at 10pts./decade with a 20 s delay and 10 s averaging time per point. Again, weight fractions are reported due to particle swelling or porosity. Limiting  $\phi_J$  ( $\phi_m = 0.447 \pm 0.003$  and  $\phi_{rcp} = 0.530 \pm 0.002$ ) were determined using the same method as §S2, with steady high-stress viscosities seen for  $\phi \leq 0.44$ . Fitting the  $\eta_r(\sigma)$  relation using corrected stresses, Eq. S6, we find  $\sigma^* = 2.3 \text{ Pa}$  and  $\beta = 0.94$ , which gives  $\phi_{DST} = 0.436$ . Time-dependent measurements were made using a TA Instruments DHR-2 with roughened plates ( $R = 20 \text{ mm}$  and  $h = 1.5 \text{ mm}$ ), as for the 50 wt.% glycerol-water cornstarch suspension.

## B. Cornstarch in 85 wt. % glycerol

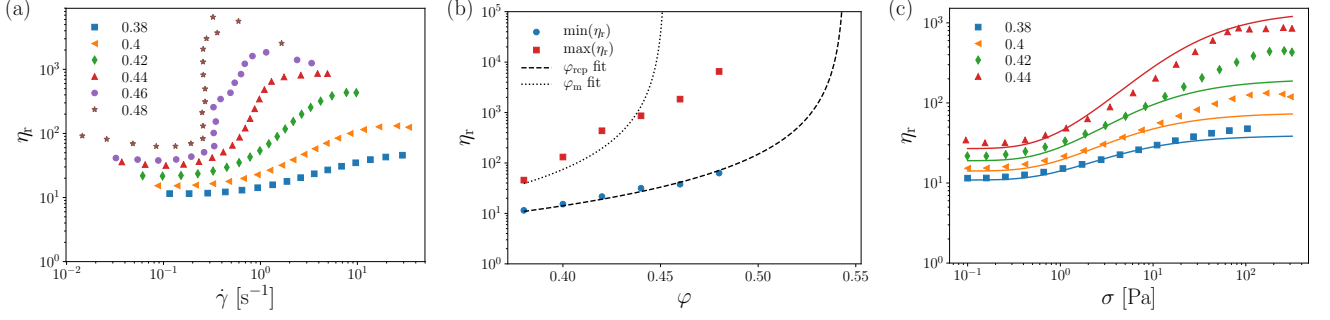

FIG. S5. Steady-state shear rheology of a cornstarch suspension in 85 wt.% glycerol-water background solvent. (a) Flow curves: relative viscosity,  $\eta_r$ , *vs.* shear rate,  $\dot{\gamma}$ , for multiple weight fractions,  $\phi$ , listed. (b) Maximum (red squares) and minimum (blue circles) viscosities as a function of  $\phi$ , fits to Eq. S5 are shown, with dotted and dashed black lines respectively, finding  $\phi_m = 0.452 \pm 0.004$ ,  $\phi_{rcp} = 0.545 \pm 0.003$ . (c) Corrected flow curves, relative viscosity *vs.* stress,  $\eta_r(\sigma)$ , for  $\phi < \phi_m$ , used for fitting WC model parameters:  $\beta = 0.81 \pm 0.07$  and  $\sigma^* = 1.3 \pm 0.2$ .

For the cornstarch suspensions, now in an 85 wt.% glycerol-water background solvent, slow swelling is visibly apparent over  $\sim 2$  h; for reproducibility, samples were therefore measured after  $\sim 4$  h resting, using a roller bank to prevent sedimentation. The background solvent viscosity was measured from the centrifuged supernatant of 40 wt.% samples,  $\eta_s = 75$  mPa.s, significantly lower than the 110 mPa.s viscosity measured before mixing with cornstarch. The viscosity reduction suggests the cornstarch preferentially absorbs glycerol. Otherwise, all measurements were made using the same protocol and methods as for the cornstarch suspension in a 50 wt.% glycerol-water background solvent with an increased point time, 15 s delay and 15 s average, due to the reduced shear rates.

Repeating the fitting protocol used for 50 wt.% glycerol-water suspension, §S2, we find  $\phi_m = 0.452 \pm 0.004$  and  $\phi_{rcp} = 0.545 \pm 0.003$ , from the maximum and minimum steady viscosities respectively. Again, applying Eq. S6 and fitting  $\eta_r(\sigma)$ , we find  $\beta = 0.81 \pm 0.07$  and  $\sigma^* = 1.3 \pm 0.2$ , which gives  $\phi_{DST} = 0.445$ . Time-dependent measurements were made using a TA Instruments DHR-2 with roughened plates ( $R = 20$  mm and  $h = 1.5$  mm), as for the 50 wt.% glycerol-water cornstarch suspension.

### C. Silica suspensions

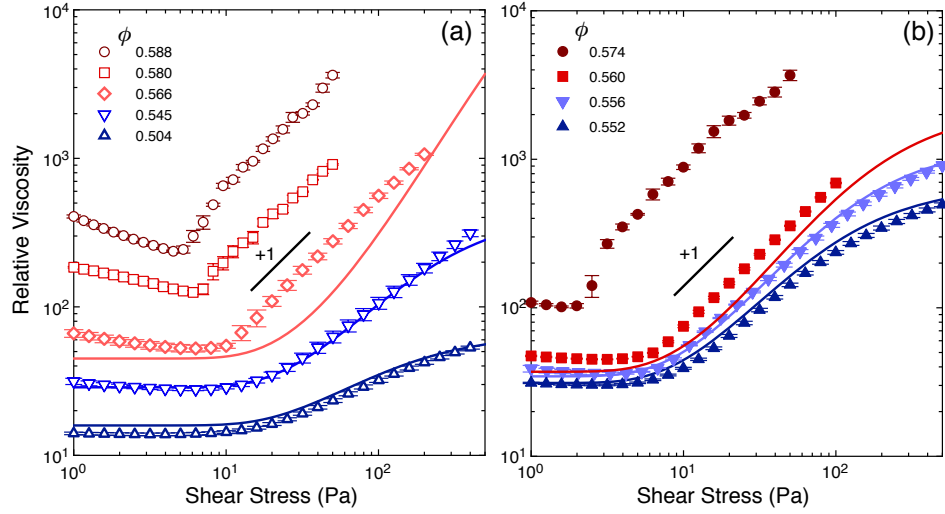

FIG. S6. Flow curves  $\eta_r(\sigma)$  for suspensions of  $d = 4.0 \mu\text{m}$  silica spheres at various volume fractions  $\phi$  suspended in: (a) 80 wt.% DMSO-water, (b) 87 wt.% glycerol-water. Error bars give the standard deviation from two up and down stress sweeps. Solid lines show Wyart-Cates flow curves with  $\phi_{\text{rcp}} = 0.67$ ,  $\phi_m = 0.57$ ,  $\sigma^* = 14.5 \text{ Pa}$  for suspensions in DMSO-water and  $\sigma^* = 40.0 \text{ Pa}$  for suspensions in glycerol-water.

Suspensions of silica spheres (AngstromSpheres, Blue Helix UK) with a mean diameter  $d = 4.0 \mu\text{m}$ , (measured from SEM images of dried particles) were prepared in either an 87 wt.% glycerol-water mixture ( $\eta_s = 151 \text{ mPa}\cdot\text{s}$  at  $20^\circ\text{C}$ ) or an 80 wt.% dimethyl sulfoxide (DMSO) - water mixture ( $\eta_s = 3.4 \text{ mPa}\cdot\text{s}$ ). These fluid compositions were chosen to nearly match the refractive index of the silica particles ( $n = 1.454$ ), minimizing attractive van der Waals interactions between particles. To prepare suspensions, we first dispersed dry particles in water using a combination of mechanical mixing and probe ultrasonication to break up aggregates present in the dry powder. We used distilled water adjusted to a pH of 9.0 using NaOH in order to increase the silica surface charge and aid dispersion. Particles were washed three times in the pH=9 distilled water by sedimentation and discarding excess supernatant, then either DMSO or glycerol was added to obtain the desired fluid composition, along with 0.2 mM fluorescein sodium salt, giving a Debye screening length  $\lambda_D \simeq 12 \text{ nm}$ . Particles were allowed to sediment a final time to prepare concentrated stock solutions for both DMSO-water and glycerol-water suspensions, and samples at varying mass fractions were prepared via dilution. Mass fractions were converted to volume fractions,  $\phi$ , using the silica particle density  $\rho_p = 2.07 \text{ g/cm}^3$ , which we determined from a series of density measurements (Anton Paar DMA 4500) with dilute suspensions of known mass fraction.

We characterized the rheology of these silica suspensions using an Anton Paar MCR 302 rheometer with sandblasted parallel plates ( $R = 20 \text{ mm}$ ) and a  $h = 1.5 \text{ mm}$  gap height. Steady-state flow curves  $\eta_r(\sigma)$ , Fig. S6, were obtained by averaging the shear rate over 20 s under fixed apparent stress, allowing us to obtain smooth flow curves even after the onset of oscillations in the silica-DMSO/water suspensions. While the value of the onset stress  $\sigma^*$  was lower in the DMSO-water suspensions than in the glycerol-water suspensions (14.5 Pa vs 40.0 Pa), we found the flow curves could be reasonably well fit with a fixed  $\phi_{\text{rcp}} = 0.67$  and  $\phi_m = 0.57$  for both systems.

## S6. GAP HEIGHT VARIATION

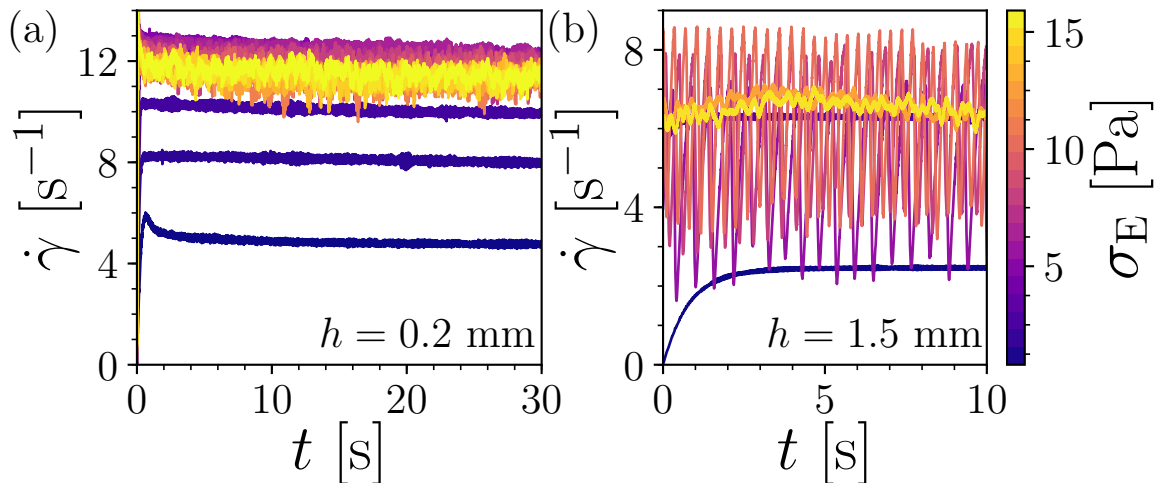

FIG. S7. Effect of gap height variation on time-dependent flow under constant external stress for a  $\varphi = 0.47$  cornstarch suspension in 50 wt.% glycerol-water. (a) Gap height,  $h = 0.2$  mm, other experimental parameters unchanged from Fig. 3(a) giving  $\epsilon = 2.0 \times 10^{-5} \approx \epsilon_c^{\max}$ . Traces are taken at 250 Hz, over 30 s constant imposed external stress,  $\sigma_E$ , in 0.8 Pa steps from 0 to 16 Pa, see color bar (right). (b)  $h = 1.5$  mm, otherwise as in (a). For clarity, only every third stress has been plotted over the first 10 s of the 30 s step.

Previously, we explored variation of the background solvent viscosity (§5),  $\eta_s$ , and the effect on the presence of oscillations, see Main Text.  $\epsilon$ , however, has multiple parameters. While some are (to our knowledge) fixed ( $\gamma_0$ ), or set mainly by particle size ( $\sigma^*$ ) [2],  $h$  and  $\rho_A$  should be variable. Unlike  $\eta_s$ , however, they enter  $\epsilon$  *linearly*, making substantial variation of  $\epsilon$  challenging. To increase  $\epsilon$ , the gap height is decreased. We focus on a  $\varphi = 0.47$  cornstarch suspension at  $h = 1.5$  mm showed large amplitude oscillations, Fig. 3(a), over the greatest range of stresses, Fig. 4. Therefore, if oscillations are suppressed at  $\varphi = 0.47$  it is highly likely they are suppressed over the whole range of  $\varphi$ .

Decreasing  $h$  to 0.2 mm from 1.5 mm increases  $\epsilon$  from  $2.7 \times 10^{-6}$  to  $2.0 \times 10^{-5} \approx \epsilon_c^{\max}$ . Applying constant  $\sigma_E$  for 30 s steps from 0 to 16 Pa in 0.8 Pa steps, we see no shear-rate oscillations, Fig. S7(a), in contrast to the same  $\varphi$  with  $h = 1.5$  mm, Fig. S7(b). This is despite the continued presence of DST ( $\dot{\gamma}$  decreasing with stress from magenta to yellow traces). This is not inconsistent with the prediction of the model. We note, however, that this gap height is approaching a small number of particle diameters,  $\mathcal{O}(10)$ , and that therefore there may be additional effects, from, *e.g.*, plate roughness, geometry misalignment and excluded volume effects changing the effective  $\varphi$  [3]. We therefore do not present a more systematic investigation of the effect of gap height.

As mentioned above,  $\rho_A$  could in theory also be varied. Although, in practice, while the contribution to  $\rho_A$  from the tool (*i.e.* the plate in contact with the sample) can be substantially varied (*e.g.* changing radius, material, from parallel plate to cone-plate or Couette cylinder, *etc.*) the internal inertia of the rheometer, which applies the torque to the tool, cannot be varied. This prevents a large decrease of  $\rho_A$  within the range of standard rheometric geometries, and it is not possible to sufficiently decrease  $\epsilon$ . Correspondingly oscillations have been observed in multiple standard geometries [1].

## S7. EFFECT OF TIME-DEPENDENT RELAXATION

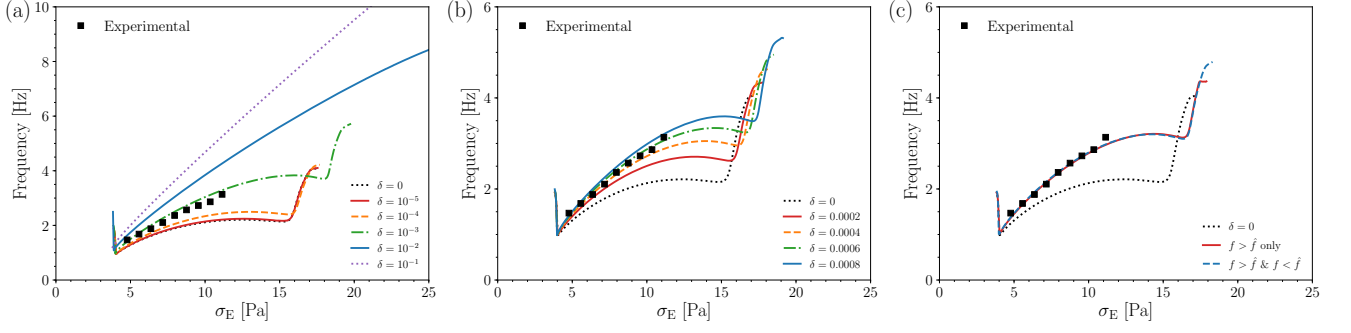

FIG. S8. Effect of time-dependent relaxation, oscillation frequency as a function of applied stress,  $\sigma_E$ . Stress-frequency dependence for strain dependent relaxation only included for comparison (dotted black line). (a) Varying relaxation rate,  $\delta$ , over multiple orders of magnitude, showing sensitivity of the stress-dependent frequency to  $\delta$  between  $\delta \sim 10^{-5}$  and  $\delta \sim 10^{-1}$ . Lines, frequency of model with labelled  $\delta$  and other parameters:  $\epsilon = 2.7 \times 10^{-6}$ ,  $\varphi_m = 0.457$ ,  $\varphi_{rcp} = 0.546$ ,  $\beta = 0.94$ .  $\sigma^* = 5.5$  Pa,  $\eta_s = 6$  mPa s,  $\rho_A = 175$  kg m $^{-2}$  and  $h = 1.5$  mm used to non-dimensionalise. Points, experimental data for  $\varphi = 0.47$ . (b) Fine variation of  $\delta$ , 0.0002 to 0.0008, parameters and data as in (a). (c) Impact of restricting time-dependent relaxation to  $f > \hat{f}$ .  $\delta = 5 \times 10^{-4}$ , other parameters as in (a), comparison of time dependent relaxation only applying when  $f > \hat{f}$  (red, solid line) and for all  $f$  values (blue, dashed line).

Eq. 11, introducing explicitly time-dependent  $f$ -relaxation, can also be non-dimensionalized using the inertial time scale,  $t_i$ ,

$$\epsilon \frac{df}{d\tau} = - \left( \dot{\Gamma} + \delta \right) \left[ f - \hat{f}(\eta_r(f)\dot{\Gamma}) \right], \quad (\text{S10})$$

introducing a dimensionless relaxation rate,  $\delta = \gamma_0 \eta_s / (t_r \sigma^*)$ . When  $\dot{\Gamma}$  drops close to 0 during the limit cycle, the relaxation of  $f$  towards its steady-state value is increased by  $\delta$ . At high values of  $\delta$ , relaxation will be dominated by the time-dependent term, making section  $DA$  of the limit cycle fast in time, not just strain. As the section  $DA$  of the limit cycle becomes fast it will make up a small proportion of the total limit cycle time, now dominated by  $AB$ . Further increasing  $\delta$  will then not significantly increase the frequency, creating a range of sensitivity for measuring the relaxation rate between  $\delta \sim 10^{-5}$  and  $\delta \sim 10^{-1}$ , Fig. S8(a), corresponding to relaxation times  $t_r \sim 10$  s to  $t_r \sim 10^{-3}$  s.

Varying  $\delta$  across a more narrow range,  $2 \times 10^{-4}$  to  $8 \times 10^{-4}$ , see Fig. S8(b), for  $\sigma_E > 6$  Pa, the data points, including those for  $\varphi = 0.48$  (not shown for clarity), lie between the lines for  $\delta = 4 \times 10^{-4}$  and  $\delta = 6 \times 10^{-4}$ ; we therefore quote  $\delta = 5 \pm 1 \times 10^{-4}$ , corresponding to  $t_r = 0.24(5)$  s.

In Eq. 11 time-dependent relaxation of  $f$  towards  $\hat{f}$  occurs for both  $f > \hat{f}$  and  $f < \hat{f}$ , however as we are aiming to capture inherent relaxation of bonds *after* they have been formed, due to *e.g.* repulsion, softness or relaxation of polymers on the surface, we should only consider  $f > \hat{f}$ . As  $\delta$  is small it only acts significantly close to jamming, *i.e.* when  $\dot{\Gamma} \lesssim \delta$ . Time-dependent relaxation will then only be significant when  $f > \hat{f}$  anyway, see Fig. 2(d). We can therefore use Eq. 11 without specifying  $f > \hat{f}$ , making no impact on the measured frequency, Fig. S8(c).

## S8. BEHAVIOR AT THE ONSET OF INSTABILITY

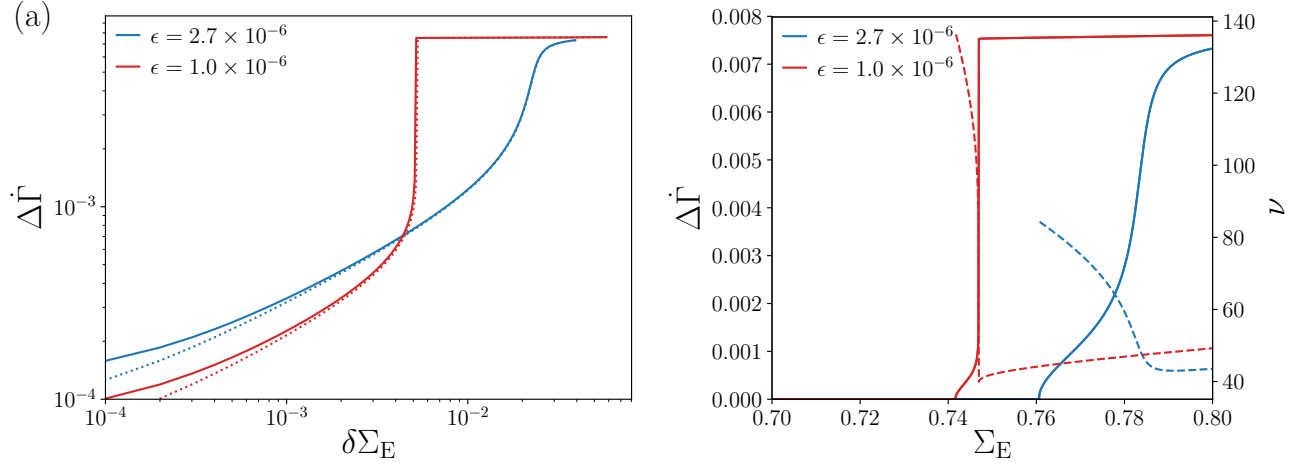

FIG. S9. behavior of limit cycle at onset of instability. (a) Amplitude,  $\Delta \dot{\Gamma}$ , as a function of applied stress above the onset of instability,  $\delta \Sigma_E$ , at  $\varphi = 0.47$  for two different  $\epsilon$  values: blue,  $\epsilon = 1.0 \times 10^{-6}$ ; red,  $\epsilon = 2.7 \times 10^{-6}$ . WC model parameters as in main text:  $\varphi_{\text{rcp}} = 0.546$ ,  $\varphi_m = 0.457$ ,  $\beta = 0.94$ . Stress difference calculated from the amplitude of the first non-zero oscillation, defined as  $\Delta \dot{\Gamma} > 10^{-7}$ . Solid lines, increasing stress sweep; dotted lines, decreasing stress sweep for 1000 steps between  $\Sigma_E = 0.7$  and  $0.8$  taking initial conditions from the previous step. (b) Amplitude (solid lines) and frequency ( $\nu$ , dashed lines) as a function of applied stress,  $\Sigma_E$ . Colors and parameters as in (a).  $\nu$  is measured in units of reciprocal dimensionless time,  $\tau^{-1} = t_i/t$ .

In our model, instability sets in above discontinuous shear thickening (where  $d\dot{\Gamma}/d\Sigma_E = 0$ ), at a (dimensionless) applied stress,  $\Sigma_E^0$ , when  $-\dot{\Gamma}d\dot{\Gamma}/d\Sigma_E = \epsilon$ , Fig. 2(b). Figure S9(a) shows how the predicted amplitude of the shear rate oscillations,  $\Delta \dot{\Gamma} = \max(\dot{\Gamma}) - \min(\dot{\Gamma})$ , increases as the stress increases beyond this point in the vicinity of the threshold, to  $\Sigma_E^0 + \delta \Sigma_E$ , at two values of  $\epsilon$ . Just above the onset of instability,  $0 < \delta \Sigma_E \lesssim 10^{-3}$ , additional applied stress causes a slow increase in amplitude, consistent with a supercritical Hopf bifurcation. Sweeping the applied stress up (solid lines) and then down (dotted lines), we found no evidence of hysteresis. The small differences between the up and down sweeps at low  $\delta \Sigma_E$  are due to the precision in numerically determining the onset of instability.

Figure S9(b) shows the evolution of the oscillation amplitude (continuous lines) and frequency (measured in units of reciprocal dimensionless time,  $\tau^{-1} = t_i/t$ , dashed lines) as a function of  $\Sigma_E$ . We see that the small-amplitude oscillations in the vicinity of the threshold have high frequencies. The frequency then decreases as the amplitude increases with increasing applied stress, although the manner of this transition depends on  $\epsilon$ . For  $\epsilon = 2.7 \times 10^{-6}$ ,  $\Delta \dot{\Gamma}$  increases smoothly to its saturation value, whereas for  $\epsilon = 1 \times 10^{-6}$  there is a sudden jump in amplitude to a plateau. Decreasing  $\epsilon$  from  $2.7 \times 10^{-6}$  to  $1.0 \times 10^{-6}$  also reduces the range of stresses for small-amplitude high-frequency oscillations, which additionally have even higher frequencies. The very small range of stresses over which these higher frequencies oscillations are predicted to occur means that they will not be observed in experiments. In practice, Fig. S8, observed oscillations have a frequency that increases slowly with applied stress, as predicted for low  $\epsilon$  values after the sharp drop in  $\nu(\Sigma_E)$  at the onset, Fig. S9(b) (red dashed line).

- 
- [1] M. Hermes, B. M. Guy, W. C. K. Poon, G. Poy, M. E. Cates, and M. Wyart, *J. Rheol.* **60**, 905 (2016).
  - [2] B. M. Guy, M. Hermes, and W. C. K. Poon, *Phys. Rev. Lett.* **115**, 088304 (2015).
  - [3] Y. Madraki, G. Ovarlez, and S. Hormozi, *Phys. Rev. Lett.* **121**, 108001 (2018).
